# Supplementary material for: Controlling for sparsity in sparse factor analysis models: adaptive latent feature sharing for piecewise linear dimensionality reduction
Source: arXiv:2006.12369 source file (2021-02-28)
Supplement: Supplementary file 1 [file Supplementary_material.pdf]

# Supplementary material.

**Adam Farooq**
Aston University

**Yordan P. Raykov**
Aston University

**Max A. Little**
University of Birmingham

**César Michelet**
ENSIIE

## 1 Inference

### 1.1 Collapsed Gibbs inference

The posterior of the $k^{th}$ direction $\mathbf{w}_k$ is:

$$\begin{gathered}\mathrm{P}\left(\mathbf{w}_k|\mathbf{Y},\mathbf{Z},\mathbf{W}^{(\neg k)},\sigma_y,\sigma_x\right)\\ \propto \mathrm{P}\left(\mathbf{w}_k\right)\times\mathrm{P}\left(\mathbf{Y}|\mathbf{W},\mathbf{Z},\sigma_y,\sigma_x\right)\\ \propto \exp\left(\mathbf{w}_k^T\left(\frac{\sigma_x^2\sum_{n=1}^N z_{kn}\mathbf{y}_n\mathbf{y}_n^T}{2\sigma_y^2\left(\sigma_y^2+\sigma_x^2\right)}\right)\mathbf{w}_k\right)\end{gathered}$$

if we set $\mathbf{w}_k=\mathbf{B}\mathbf{v}_k$, then the posterior of $\mathbf{w}_k$ can be re-written as:

$$\begin{gathered}\mathrm{P}\left(\mathbf{w}_k|\mathbf{Y},\mathbf{Z},\mathbf{W}^{(\neg k)},\mathbf{B},\sigma_y,\sigma_x\right)\\ \propto \exp\left(\mathbf{v}_k^T\mathbf{B}^T\left(\frac{\sigma_x^2\sum_{n=1}^N z_{kn}\mathbf{y}_n\mathbf{y}_n^T}{2\sigma_y^2\left(\sigma_y^2+\sigma_x^2\right)}\right)\mathbf{B}\mathbf{v}_k\right)\end{gathered}$$

which can be re-written as:

$$\begin{gathered}\mathrm{P}\left(\mathbf{v}_k|\mathbf{Y},\mathbf{Z},\mathbf{W}^{(\neg k)},\mathbf{B},\sigma_y,\sigma_x\right)\\ \propto \exp\left(\mathbf{v}_k^T\mathbf{B}^T\left(\frac{\sigma_x^2\sum_{n=1}^N z_{kn}\mathbf{y}_n\mathbf{y}_n^T}{2\sigma_y^2\left(\sigma_y^2+\sigma_x^2\right)}\right)\mathbf{B}\mathbf{v}_k\right)\end{gathered}$$

this implies that we can simply draw $\mathbf{v}_k$ from the Bingham distribution with parameters $\left(\mathbf{B}^T\left(\frac{\sigma_x^2\sum_{n=1}^N z_{kn}\mathbf{y}_n\mathbf{y}_n^T}{2\sigma_y^2\left(\sigma_y^2+\sigma_x^2\right)}\right)\mathbf{B}\right)$, and set $\mathbf{w}_k=\mathbf{B}\mathbf{v}_k$; this will ensure that $\mathbf{w}_k$ is still orthornomal to the existing $(D-K^+-1)$ directions in $\mathbf{W}^{(\neg k)}$.

### 1.2 Collapsed Gibbs Algorithm

The collapsed Gibbs pseudocode can be seen below in Algorithm 1 where $\mathrm{V}(d)$ is the uniform distribution on a $d$-dimensional unit hypersphere andOrth $(\cdot)$ represents the orthornomal basis of a matrix and $\mathbf{\Theta}=\{\sigma_y,\sigma_x,\alpha\}$.

### 1.3 Maximization-Expectation-Maximization (MEM) derivation

The likelihood of the model is:

**Algorithm 1** Collapsed Gibbs pseudocode for A-PPCA

```
Input: Y, Θ, MaxIter, σ_MH
Initialise: Set K+ = 1
for iter ← 1 to MaxIter
  if iter=1
    Sample v ∼ V(D − 1)
    Set w_1 = v
  for n ← 1 to N
    for k ← 1 to K+
      Sample z_kn ∼ Bern( eq(7) / (eq(7)+eq(8)) )
      Sample κ ∼Poisson(α/N)
      if κ > 1
        K+_prop = K+, W_prop = [ ]
        for i ← 1 to κ
          K+_prop = K+_prop + 1
          Set B= Orth([W, W_prop]^⊥)
          Sample v ∼V(D − K+_prop)
          Update W_prop = [W_prop, Bv]
        if eq (15)> Uniform([0,1]) / Uniform([0,1])
          Set W = [W, W_prop] and K+ = K+ + K+_prop
  for j ← 1 to K+
    Set B= Orth([w_1, ..., w_{j−1}, w_{j+1}, ..., w_{K+}]^⊥)
    Sample v ∼ Bingham( B^T ( σ_x^2 Σ_{n=1}^N z_kn y_n y_n^T / (2σ_y^2(σ_y^2+σ_x^2)) ) B )
    Update w_j = Bv
  Sample Θ using Metropolis-Hastings
Output: Z, Θ
```

$$\begin{gathered}\mathrm{P}\left(\mathbf{Y}|\mathbf{Z},\mathbf{W},\mathbf{X},\sigma_x,\sigma_y\right)\times\mathrm{P}\left(\mathbf{X}\right)\times\mathrm{P}\left(\mathbf{W}\right)\\ =\frac{1}{\left(2\pi\sigma_y^2\right)^{ND/2}}\frac{1}{\left(2\pi\sigma_x^2\right)^{NK^+/2}}\prod_{k=1}^{K^+}\frac{\Gamma\left(\frac{D-(k-1)}{2}+1\right)}{\pi^{(D-(k-1))/2}}\\ \times\prod_{n=1}^N\exp\left(-\frac{1}{\left(2\sigma_y^2\right)}\left(\mathbf{y}_n^T-\sum_{k=1}^{K^+}\left(z_{kn}x_{kn}\mathbf{w}_k^T\right)\right)\right.\\ \left.\times\left(\mathbf{y}_n-\sum_{k=1}^{K^+}\left(\mathbf{w}_k z_{kn}x_{kn}\right)\right)-\frac{1}{\left(2\sigma_x^2\right)}\sum_{k=1}^{K^+}\left(x_{kn}^2\right)\right)\end{gathered}$$

then we use the log-likelihood $\mathcal{L}_N=\ln\left(\mathrm{P}\left(\mathbf{Y}|\mathbf{Z},\mathbf{W},\mathbf{X},\sigma_x,\sigma_y\right)\times\mathrm{P}\left(\mathbf{X}\right)\times\mathrm{P}\left(\mathbf{W}\right)\right)$, $\mathbf{w}_k^T\mathbf{w}_n=0$ for $k\neq n$, and we also take the expectation with respect to the distributions $\mathrm{P}\left(x_{kn}|\mathbf{y}_n,\mathbf{w}_k,z_{kn},\sigma_y,\sigma_x\right)$:

$$\begin{aligned}\mathcal{L}_N = & -\tfrac{NK^+}{2}\ln\left(2\pi\sigma_x^2\right) - \tfrac{ND}{2}\ln\left(2\pi\sigma_y^2\right) \\ & -\textstyle\sum_{n=1}^{N}\Bigg(\tfrac{1}{2\sigma_y^2}\mathbf{y}_n^T\mathbf{y}_n + \textstyle\sum_{k=1}^{K^+}\Big(\tfrac{1}{2\sigma_x^2}\left\langle x_{kn}^2\right\rangle \\ & -\tfrac{1}{\sigma_y^2}\left(z_{kn}\left\langle x_{kn}\right\rangle\mathbf{w}_k^T\right)\mathbf{y}_n + \tfrac{1}{2\sigma_y^2}\left(z_{kn}\left\langle x_{kn}^2\right\rangle\mathbf{w}_k^T\mathbf{w}_k\right)\Big)\Bigg)\end{aligned} \tag{1}$$

where terms independent of the model parameters have been omitted and:

$$\begin{aligned}\left\langle x_{kn}\right\rangle &= \left(\frac{1}{\sigma_x^2}+\frac{1}{\sigma_y^2}z_{kn}\right)^{-1}\left(\frac{1}{\sigma_y^2}z_{kn}\mathbf{w}_k^T\mathbf{y}_n\right) \\ \left\langle x_{kn}^2\right\rangle &= \left(\frac{1}{\sigma_x^2}+\frac{1}{\sigma_y^2}z_{kn}\right)^{-1} + \left\langle x_{kn}\right\rangle\end{aligned}$$

Our first goal is to maximize equation (1) with respect to $\mathbf{w}_k$, but in order to ensure that the orthornomality in the columns of $\mathbf{W}$ remains, $\mathbf{w}_k$ can be re-written as $\mathbf{w}_k = \mathbf{B}\mathbf{v}_k$,where $\mathbf{B}$ is a $(D \times (D - K^+ + 1))$ matrix containing the orthonormal basis of all $(D - K^+ + 1)$ directions which are orthogonal to the matrix $\mathbf{W}^{(\neg k)} = [\mathbf{w}_1, \ldots, \mathbf{w}_{k-1}, \mathbf{w}_{k+1}, \ldots, \mathbf{w}_{K^+}]$, then:

$$\begin{aligned}\tfrac{\partial\mathcal{L}_N}{\partial\mathbf{v}_k} = & \textstyle\sum_{n=1}^{N}\left(\tfrac{1}{\sigma_y^2}z_{kn}\left\langle x_{kn}\right\rangle\mathbf{B}^T\mathbf{y}_n\right) \\ & -\textstyle\sum_{n=1}^{N}\left(\tfrac{1}{\sigma_y^2}z_{kn}\left\langle x_{kn}^2\right\rangle\mathbf{B}^T\mathbf{B}\mathbf{v}_k\right)\end{aligned} \tag{2}$$

as $\mathbf{B}^T\mathbf{B} = \mathbb{I}_{K^+}$ and by setting equation (2) to zero, the optimal solution for $\mathbf{v}_k$ and $\mathbf{w}_k$ is:

$$\begin{aligned}\mathbf{v}_k &= \left(\frac{1}{\sigma_y^2}\sum_{n=1}^{N}z_{kn}\left\langle x_{kn}\right\rangle\mathbf{B}^T\mathbf{y}_n\right)\left(\frac{1}{\sigma_y^2}\sum_{n=1}^{N}z_{kn}\left\langle x_{kn}^2\right\rangle\right)^{-1} \\ \mathbf{w}_k &= \mathbf{B}\left(\frac{1}{\sigma_y^2}\sum_{n=1}^{N}z_{kn}\left\langle x_{kn}\right\rangle\mathbf{B}^T\mathbf{y}_n\right)\left(\frac{1}{\sigma_y^2}\sum_{n=1}^{N}z_{kn}\left\langle x_{kn}^2\right\rangle\right)^{-1}\end{aligned}$$

By setting $\frac{\partial\mathcal{L}_N}{\partial\sigma_y}$ to zero, we obtain the following solution for $\sigma_y^2$:

$$\begin{aligned}\sigma_y^2 = & \tfrac{1}{ND}\textstyle\sum_{n=1}^{N}\Bigg(\mathbf{y}_n^T\mathbf{y}_n - \\ & -2\textstyle\sum_{k=1}^{K^+}\left(z_{kn}\left\langle x_{kn}\right\rangle\mathbf{w}_k^T\mathbf{y}_n + \left\langle x_{kn}^2\right\rangle\right)\Bigg)\end{aligned}$$

By setting $\frac{\partial\mathcal{L}_N}{\partial\sigma_x}$ to zero, we obtain the following solution for $\sigma_x^2$:

$$\sigma_x^2 = \frac{1}{NK^+}\sum_{n=1}^{N}\left(\sum_{k=1}^{K^+}\left\langle x_{kn}^2\right\rangle\right)$$
